# Supplementary material for: Implicit Filter Sparsification In Convolutional Neural Networks
Source: arXiv:1905.04967 source file (2019-05-13)
Supplement: Supplementary file 1 [file layerwise_sparsity_cifar100_supp.tex]

%%!TEX root = ../supp_article.tex

%\begin{table*}[]
\begin{table*}[]
\centering
\caption{Layerwise \% filters pruned from BasicNet trained on CIFAR100, based on the $|\gamma| <10^{-3}$ criteria. Also shown are pre-pruning and post-pruning test error. C1-C7 indicate Convolution layer 1-7, and the numbers in parantheses indicate the total number of features per layer. Average of 3 runs.}
%\kimki{I guess we do not need to use resize box for the tables that are smaller than the column or row width.}}
\label{tbl:layerwise_sparsity_leaky}
%\resizebox{0.9\linewidth}{!}{
\begin{tabular}{lccccccccccccc}
                                             \multicolumn{5}{l|}{\textbf{Adam vs AMSGrad (ReLU)}}                      & \multicolumn{8}{c|}{\% Sparsity by $\gamma$ or \% Filters Pruned}                                                                                                                                                                &                                            \multicolumn{1}{l}{}         \\ \cline{6-13}
                       & \multicolumn{1}{l|}{}         &    Train                  & \multicolumn{1}{c|}{Test}          & \multicolumn{1}{c|}{Test}          & \T C1                   & C2                   & C3                   & C4                   & C5                   & C6                   & \multicolumn{1}{c|}{C7}    & \multicolumn{1}{c|}{Total}                                               & Pruned                       \\
               & \multicolumn{1}{l|}{}         & Loss           & \multicolumn{1}{c|}{Loss} & \multicolumn{1}{c|}{Err}  & (64)                 & (128)                & (128)                & (256)                & (256)                & (512)                & \multicolumn{1}{c|}{(512)} & \multicolumn{1}{c|}{(1856)}                                            & Test Err.                    \\ \hline
\multicolumn{1}{|l}{}                       & \multicolumn{1}{|c|}{\T L2: 1e-3} & 1.06                 & \multicolumn{1}{c|}{1.41}      & \multicolumn{1}{c|}{39.0}      & 56                   & 47                   & 43                   & 68                   & 72                   & 91                   & \multicolumn{1}{c|}{85}    & \multicolumn{1}{c|}{76}                             & 39.3 \\
\multicolumn{1}{|c}{\multirow{-2}{*}{\rotatebox[origin=c]{90}{Adam}}}                       & \multicolumn{1}{|c|}{L2: 1e-4 \B} & 0.10                 & \multicolumn{1}{c|}{1.98}      & \multicolumn{1}{c|}{36.6}      & 41                   & 20                   & 9                    & 33                   & 34                   & 67                   & \multicolumn{1}{c|}{55}    & \multicolumn{1}{c|}{47}                            & 36.6 \\ \hline 
\multicolumn{1}{|l}{}                       & \multicolumn{1}{|c|}{\T L2: 1e-2} & 3.01                 & \multicolumn{1}{c|}{2.87}      & \multicolumn{1}{c|}{71.9}      & 79                   & 91                   & 91                   & 96                   & 96                   & 98                    & \multicolumn{1}{c|}{96}    & \multicolumn{1}{c|}{95}                             & 71.9 \\
\multicolumn{1}{|l}{}                       & \multicolumn{1}{|c|}{\T L2: 1e-4} & 0.04                 & \multicolumn{1}{c|}{1.90}      & \multicolumn{1}{c|}{35.6}      & 0                    & 0                    & 0                    & 0                    & 1                    & 25                    & \multicolumn{1}{c|}{23}     & \multicolumn{1}{c|}{13}                               & 35.6 \\  
\multicolumn{1}{|c}{\multirow{-3}{*}{\rotatebox[origin=c]{90}{AMSGrad}}}  & \multicolumn{1}{|c|}{\T L2: 1e-6\B} & 0.01                 & \multicolumn{1}{c|}{3.23}      & \multicolumn{1}{c|}{40.2}      & 0                    & 0                    & 0                   & 0                    & 0                    & 0                    & \multicolumn{1}{c|}{0}     & \multicolumn{1}{c|}{0}                               & 40.2 \\ \hline
\end{tabular}
%}
%\resizebox{0.9\linewidth}{!}{
\begin{tabular}{ccccccccccccc}
\\
                                             \multicolumn{4}{l|}{\textbf{Adam With Leaky ReLU}}             & \multicolumn{8}{c|}{\% Sparsity by $\gamma$ or \% Filters Pruned}                                                                                                                                                                &                                            \multicolumn{1}{l}{}         \\ \cline{5-12}
                        \multicolumn{1}{l|}{}         &    Train                  & \multicolumn{1}{c|}{Test}          & \multicolumn{1}{c|}{Test}          & \T C1                   & C2                   & C3                   & C4                   & C5                   & C6                   & \multicolumn{1}{c|}{C7}    & \multicolumn{1}{c|}{Total}                                               & Pruned                       \\
                \multicolumn{1}{l|}{NegSlope=0.01}         & Loss           & \multicolumn{1}{c|}{Loss} & \multicolumn{1}{c|}{Err}  & (64)                 & (128)                & (128)                & (256)                & (256)                & (512)                & \multicolumn{1}{c|}{(512)} & \multicolumn{1}{c|}{(1856)}                                            & Test Err.                    \\ \hline
 \multicolumn{1}{c|}{L2: 1e-3} & 1.07                 & \multicolumn{1}{c|}{1.41}      & \multicolumn{1}{c|}{39.1}      & 49                   & 40                   & 39                   & 62                   & 61                   & 81                   & \multicolumn{1}{c|}{85}    & \multicolumn{1}{c|}{70}                             & 39.4 \\
 \multicolumn{1}{c|}{L2: 1e-4} & 0.10                 & \multicolumn{1}{c|}{1.99}      & \multicolumn{1}{c|}{36.8}      & 33                   & 20                   & 9                    & 31                   & 29                   & 55                   & \multicolumn{1}{c|}{53}    & \multicolumn{1}{c|}{41}                            & 36.8 \\ \hline 
 \multicolumn{13}{l}{NegSlope=0.1} \\ \hline
 \multicolumn{1}{c|}{L2: 1e-4} & 0.14                 & \multicolumn{1}{c|}{2.01}      & \multicolumn{1}{c|}{37.2}      & 38                   & 30                   & 21                    & 34                   & 31                   & 55                   & \multicolumn{1}{c|}{52}    & \multicolumn{1}{c|}{43}                            & 37.3 \\ \hline 
\end{tabular}
%}
\vspace{-0.3cm}
\end{table*}
